# Supplementary material for: Unusually High CO Abundance of the First Active Interstellar Comet
Source: arXiv:2004.09586 source file (2020-04-27)
Supplement: Supplementary file 1 [file borisov_supp_final.pdf]

# Supplementary Information

## Unusually High CO Abundance of the First Active Interstellar Comet

M. A. Cordiner et al.

# Supplementary Figures

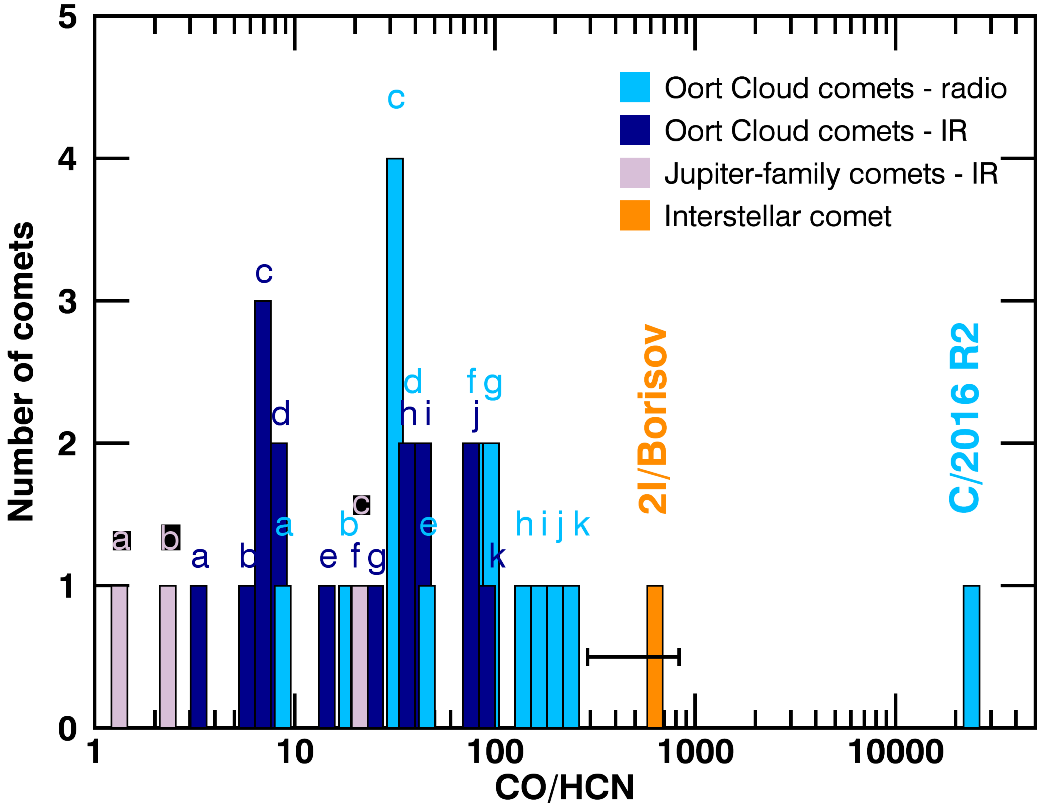


Supplementary Figure 1: Histogram (based on Figure 4), showing previously-published CO/HCN mixing ratios observed in Solar System comets [1, 2]. This version of the Figure includes alphabetical labels on the histogram bins, and the comets included in each bin are listed in Supplementary Table 2. The unusually high CO/HCN ratio of 2I/Borisov ($630^{+200}_{-340}$) is highlighted, along with the chemically peculiar outlier C/2016 R2 (PanSTARRS) (which had CO/HCN = 26,400) [3] (horizontal black bar indicates the uncertainty range of our measurement).

# Supplementary Tables

Supplementary Table 1: Mixing Ratios, $H_2O$ production Rates and Temperatures of Long-Period Cometary Comae Observed Around 2 au

| Comet | $r_H$ (au) | $T$ (K) | $Q(H_2O)$ ($s^{-1}$) | $CO/H_2O$ (%) | $HCN/H_2O$ (%) | CO/HCN | Refs. |
|---|---|---|---|---|---|---|---|
| C/1995 O1 | 2.2 | 50 | $2.4 \times 10^{29}$ | [24 ± 3] | [0.12 ± 0.01] | 200 ± 22 | [4] |
| C/1996 B2 | 1.9 | 20 | $1.2 \times 10^{29}$ | [13 ± 3] | [0.08 ± 0.01] | 162 ± 43 | [5] |
| C/2009 P1$^\dagger$ | 2.1 | 40$^*$ | $8.6 \times 10^{28}$ | 10 ± 2 | 0.28 ± 0.03 | 37 ± 8 | [6] |
| C/2009 P1$^\dagger$ | 1.7 | 50 | $1.1 \times 10^{29}$ | 19 ± 2 | 0.12 ± 0.03 | 153 ± 33 | [7] |
| C/2012 K1 | 1.8 | 42$^*$ | $3.6 \times 10^{28}$ | 3.9 ± 1 | 0.11 ± 0.02 | 36 ± 13 | [8] |
| C/2012 X1 | 1.9 | 40 | $4 \times 10^{28}$ | 32 ± 5 | 0.25 ± 0.03 | 137 ± 26 | [9] |
| 2I/Borisov | 2.0 | 50$^\ddagger$ | $6.5 \times 10^{26}$ | 68 ± 35 | 0.11 ± 0.05 | $630^{+200}_{-340}$ | [10] |

Table Footnotes — $^*$Rotational temperature of $H_2O$ (true gas kinetic temperature may be slightly higher). $^\dagger$C/2009 P1 was observed on two epochs (before and after perihelion), exhibiting relatively more CO post-perihelion. $^\ddagger$Assumed kinetic temperature. Mixing ratios in parentheses are uncertain due to non-contemporaneous $H_2O$ measurements.

Supplementary Table 2: Comets included in Figure 4 (and Supplementary Figure 1)

| Label | Jupiter-family comets |
|---|---|
| a | 103P |
| b | 73P |
| c | 9P |
| **Label** | **Oort Cloud comets - radio** |
| a | C/2007 W1 |
| b | C/2014 Q2 |
| c | C/1997 J2, C/2006 P1, C/2012 F6, C/2004 Q2 |
| d | 153P, C/1999 H1 |
| e | C/2013 R1 |
| f | C/2001 Q4, C/1998 P1 |
| g | C/1995 O1, C/2009 P1 |
| h | C/2012 X1 |
| i | C/1996 B2 |
| j | C/1999 T1 |
| k | C/2006 W3 |
| **Label** | **Oort Cloud comets - IR** |
| a | C/2000 WM1 |
| b | 8P/Tuttle |
| c | C/1999 S4, C/1999 H1, C/2006 P1 |
| d | C/2001 A2, C/2007 W1 |
| e | C/2007 N3 |
| f | C/2012 S1 |
| g | 153P |
| h | C/2004 Q2, C/2009 P1 |
| i | C/2013 R1, C/1999 T1 |
| j | C/2010 G2, C/1995 O1 |
| k | C/1996 B2 |

## References


[1] Dello Russo, N., Kawakita, H., Vervack, R. J., Weaver, H. Emerging trends and a comet taxonomy based on the volatile chemistry measured in thirty comets with high-resolution infrared spectroscopy between 1997 and 2013, *Icarus*, **278**, 301-332, (2016)

[2] Bockelée-Morvan, D. & Biver, N. The composition of cometary ices, *Philos. Trans. R. Soc. A*, **375**, 20160252, (2017)

[3] Biver, N., Bockelée-Morvan, D., Paubert, G. et al. The extraordinary composition of the blue comet C/2016 R2 (PanSTARRS), *Astron. Astrophys.*, **619**, A127, (2018)

[4] Biver, N. et al. The 1995-2002 Long-Term Monitoring of Comet C/1995 O1 (Hale-Bopp) at Radio Wavelength, *Earth, Moon, and Planets*, **90**, 5-14, (2002)

[5] Biver, N. et al. Spectroscopic Monitoring of Comet C/1996 B2 (Hyakutake) with the JCMT and IRAM Radio Telescopes, *Astrophys. J.*, **118**, 1850-1872, (1999)

[6] Villanueva, G. L. et al. A multi-instrument study of Comet C/2009 P1 (Garradd) at 2.1 AU (pre-perihelion) from the Sun, *Icarus*, **220**, 291-295, (2012)

[7] Biver, N. et al. Molecular Survey of Comet C/2009P1 (Garradd) at mm to Submm Wavelengths, in *Proceedings of the Asteroids, Comets, Meteors conference*, Niigata, Japan, LPI Contribution No. **1667**, id.6330, (2012)

[8] Roth, N. X., Gibb, E. L., Bonev, B. P. The Composition of Comet C/2012 K1 (PanSTARRS) and the Distribution of Primary Volatile Abundances among Comets, *Astron. J.*, **153**, 168, (2017)

[9] Biver, N., Agundez, M., Milam, S. Abundance of complex organic molecules in comets, in *Proceedings of the Asteroids, Comets, Meteors conference* held in Helsinki, Finland. Eds. by K. Muinonen et al., (2014)

[10] This work.
